# Supplementary material for: Blockaid: Data Access Policy Enforcement for Web Applications
Source: arXiv:2205.06911 source file (2022-06-01)
Supplement: Supplementary file 1 [file appendixStandalone.tex]

\documentclass{article}
\usepackage{xr-hyper}
\usepackage{hyperref}
\providecommand{\ifextended}{\iffalse}
\begin{document}
    \appendix
    \section{Artifact Appendix}
    \input{extendedAppendix}
\end{document}
